# Supplementary material for: From latent dynamics to meaningful representations
Source: arXiv:2209.00905 ancillary file (2024-04-09)
Supplement: Supplementary file 1 [file dAE_SI.pdf]

---

**Supplementary Information:**  
**Introducing dynamical constraints**  
**into representation learning**

---

**Dedi Wang, Yihang Wang, Luke Evans and**  
**Pratyush Tiwary**

## I. SUPPLEMENTARY METHODS

### A. Implementation details for DynamicsAE and $\beta$ -VAE

For non-image datasets, we use fully connected neural networks with 3 hidden layers and ReLU activations to parameterize the encoder and decoder. Each hidden layer in both the encoder and decoder has 32 nodes (Table 1). For image datasets, we use a convolutional neural network for the encoder and a deconvolutional neural network for the decoder. We use the same encoder/decoder architecture for  $\beta$ -VAE and DynamicsAE, shown in Table 2. The diffusion and force field in all experiments are parameterized using the same 3-layer fully connected neural networks with 64 hidden units and Tanh activation functions (Table 3). In DynamicsAE, we use 50 projections to calculate the sliced Wasserstein distances for a 2D latent space. Some other hyper-parameters are also shown in Table 4. Adam optimizers with the same learning rate of 0.001 are used to train the neural networks of both DynamicsAE and VAE.

For the hyper-parameters of DynamicsAE, the minimal distance between cluster centers  $d_{\min}$  should not be too small, ensuring there are enough samples in each bin. The hyper-parameter  $\beta$  should not be too large; otherwise, the model may ignore the input data and only focus on reducing the regularization loss, resulting in a large reconstruction error.

Supplementary Table 1: Encoder and decoder architecture for non-image datasets

| Encoder               | Decoder               |
|-----------------------|-----------------------|
| Input: $\mathbb{R}^D$ | Input: $\mathbb{R}^d$ |
| FC 32 ReLU            | FC 32 ReLU            |
| FC 32 ReLU            | FC 32 ReLU            |
| FC 32 ReLU            | FC 32 ReLU            |
| FC $d$                | FC $D$                |

### B. Three well model potential

We further demonstrate the power of our framework on a 2D three-well analytical potential with isotropic diffusion coefficient ( $M_{ij} = \delta_{ij}$ ). The governing potential is given

Supplementary Table 2: Encoder and decoder architecture for image datasets

| Encoder                                         | Decoder                                |
|-------------------------------------------------|----------------------------------------|
| Input: number of channels $\times 64 \times 64$ | Input: $\mathbb{R}^d$                  |
| $4 \times 4$ conv, 32 ReLU, stride 2            | FC 128 ReLU                            |
| $4 \times 4$ conv, 32 ReLU, stride 2            | FC $4 \times 4 \times 64$ ReLU.        |
| $4 \times 4$ conv, 64 ReLU, stride 2            | $4 \times 4$ upconv, 64 ReLU, stride 2 |
| $4 \times 4$ conv, 64 ReLU, stride 2            | $4 \times 4$ upconv, 32 ReLU, stride 2 |
| FC 128, FC $d$ or $2 \times d$                  | $4 \times 4$ upconv, 32 ReLU, stride 2 |
|                                                 | $4 \times 4$ upconv, 32 ReLU, stride 2 |

Supplementary Table 3: Architecture for learning the diffusion and force field

| Diffusion             | Force                 |
|-----------------------|-----------------------|
| Input: $\mathbb{R}^d$ | Input: $\mathbb{R}^d$ |
| FC 64 Tanh            | FC 64 Tanh            |
| FC 64 Tanh            | FC 64 Tanh            |
| FC $d$                | FC $d$                |

by:

$$\begin{aligned}
U(x, y) = & -32e^{-x^2-(y-2)^2} \\
& -32e^{-(x+1)^2-(y+\sqrt{3})^2} \\
& -32e^{-(x-1)^2-(y+\sqrt{3})^2} + 8(x^2 + y^2).
\end{aligned} \tag{1}$$

A nonlinear mapping function is used to wrap the data into a "half-moon" shape:

$$\begin{bmatrix} x' \\ y' \end{bmatrix} = f(\mathbf{X}) = \begin{bmatrix} x \\ y + x^2 \end{bmatrix}. \tag{2}$$

The overdamped Langevin simulation is performed with integration timestep of 0.001 units using the Euler-Maruyama method. A trajectory of 2,000,000 time steps is generated and saved with a temporal resolution of 0.01 units.

Supplementary Table 4: Model’s hyperparameters

| Model        | Parameter  | 3-state | aladip | dSprites | DNA   |
|--------------|------------|---------|--------|----------|-------|
| $\beta$ -VAE | $\beta$    |         |        | 4        | 10    |
|              | Batch size |         |        | 64       | 64    |
| DynamicsAE   | $\beta$    | 10      | 0.1    | 100      | 10000 |
|              | $d_{\min}$ | 5       | 3      | 5        | 5     |
|              | $L$        | 50      | 50     | 50       | 50    |
|              | Batch size | 256     | 1024   | 64       | 64    |
|              | $\gamma$   | 2       | 2      | 2        | 2     |

### C. Alanine dipeptide in water

The simulation was performed with the software GROMACS 5.0,<sup>1,2</sup> patched with PLUMED 2.4.<sup>3</sup> The temperature is kept constant at 300 K using the velocity rescaling thermostat<sup>4</sup> and the integration time step is 2 fs. A 250 ns MD trajectory is generated and the solute coordinates are stored every 0.1 ps, resulting in 2,500,000 configurations that are all aligned on the first frame using minimal root mean square deviation fit to remove global translation and rotation. The three-dimensional coordinates of the 10 heavy atoms are centered to have zero mean, and then fed into our algorithm as input.

### D. dSprites 2D shape dataset

Two generative factors (X-Position, Y-Position) of the dSprites dataset are first considered in the main text for better visualization purpose. Each of these factors has 32 values ranging from 0 to 1. To generate a long sequence of images, we take a random initial image, and sequentially transforming it according to a Gaussian random walk along the two available transformations (X-Position, Y-Position) with reflecting boundaries. The standard deviation of the Gaussian random walk is 2 while the mean is zero. A length of 12,800 image sequences is generated for analysis in this work.

Similarly, to test the performance of our algorithm on learning higher dimensional latent representation, three transformations (Scale, X-Position, Y-Position) of the dSprites dataset

are considered. Note that there are only 6 values linearly spaced in  $[0.5, 1]$  for the Scale transformation. The same Gaussian random walk is used to generate a length of 12,800 image sequences for analysis.

### E. Fluorescent DNA dataset

The dataset consisting of videos of a DNA molecule floating in solution undergoing random thermodynamic fluctuations is described in Ref. 5. In this work, we only studied the videos with no noise added ( $\sigma_e = 0V$ ), wherein the DNA molecule is undergoing a free Brownian motion without drift. A total of 68 DNA molecules are recorded at this noise intensity. However, in some videos, there are more than one DNA molecules appearing under the camera. For simplicity, we removed those videos from the dataset, and finally obtained 57 DNA movies. Following the previous study<sup>6</sup>, we use the same approach to obtain the “ground truth” latent variables (the x and y position of DNA molecule) by computing the first moment of its fluorescence intensity distribution. This position information is then used to crop and size these images to the size of  $64 \times 64$ , and a simple samplewise normalization is used to improve the contrast.

## II. SUPPLEMENTARY DISCUSSION

### A. Regular space clustering in the latent space

In this work, the regular space clustering with Euclidean distance metric is used to discretize the latent space to obtain uniformly distributed bins  $\{\mathcal{Z}_k\}_{k=1}^K$ .<sup>7</sup> A hyper-parameter  $d_{\min}$  is used to control the minimum distances between cluster centers. The final cluster centers obtained are shown in Supplementary Fig. 1.

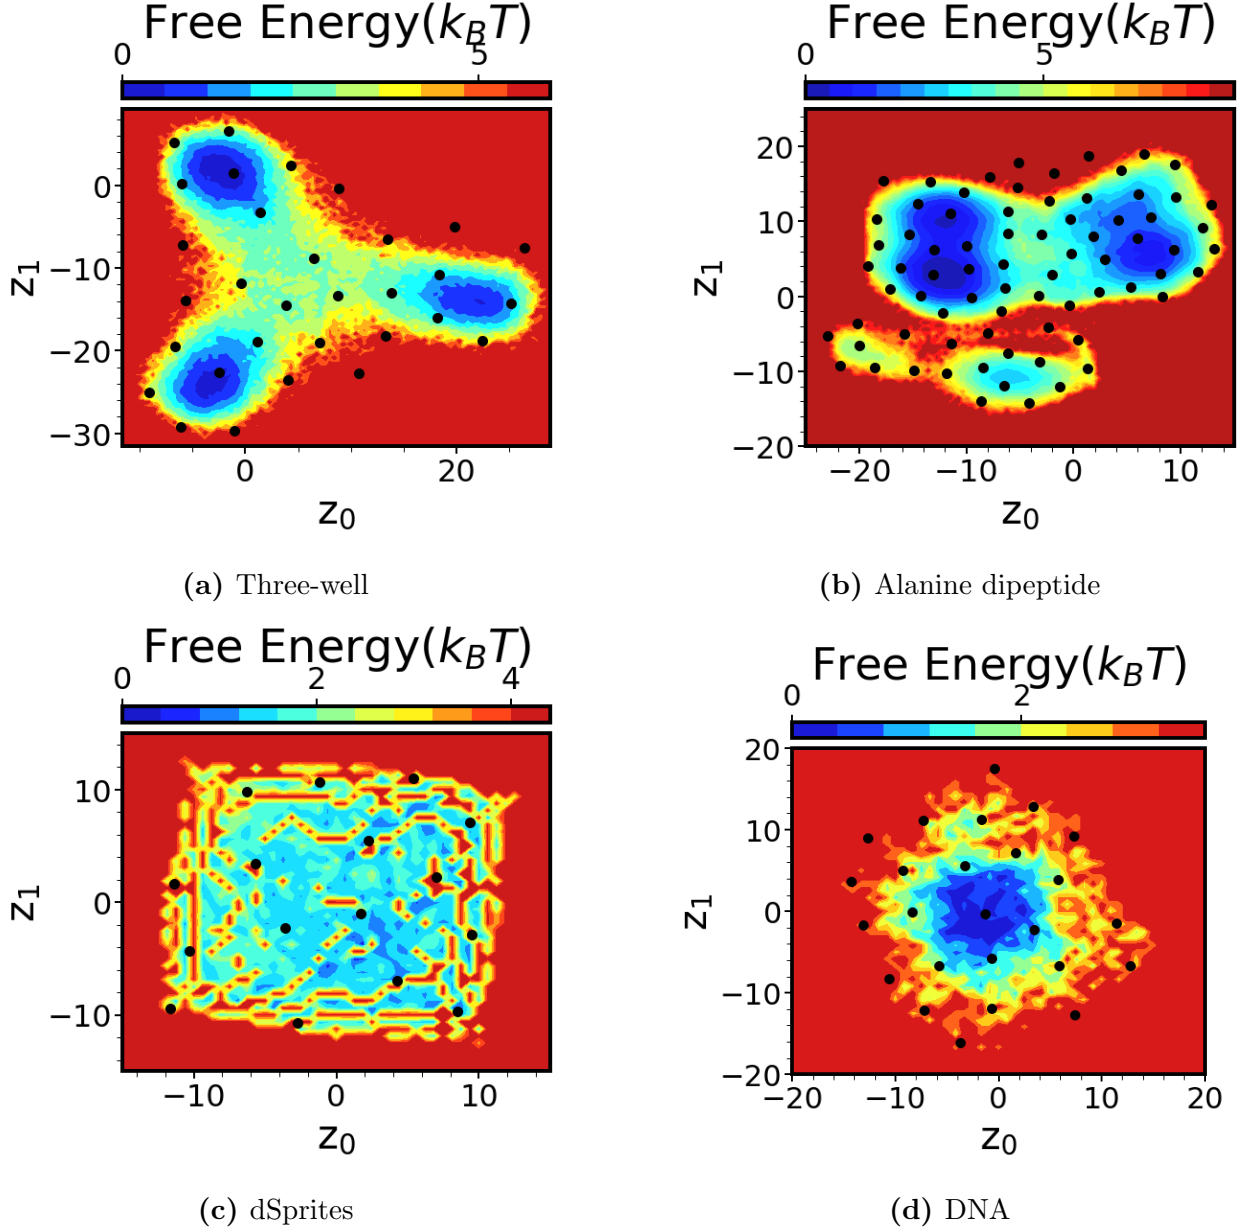

**Supplementary Figure 1:** The final cluster centers obtained using regular space clustering.

## B. Related work

Regularizing the latent space via its dynamics has started to become a topic of exploration in the past few years. Ref. 6 has similarities with our work, where the authors generalize the VAE framework to learn a latent space governed by a stochastic differential equation (SDE) with an isotropic diffusion coefficient. However, their approach still requires the

knowledge of the prior probability distribution of the latent variables, which they assume to be a Gaussian. Moreover, the authors regularize the latent space via the KL divergence between the prior distribution and the posterior distribution, which in fact cannot guarantee the latent latent space really follows the specified dynamics. In Ref. 8, a method is proposed to extend VAEs for sequential data with a latent space explicitly decomposed as position and momentum, governed by a continuous-time probabilistic ODE. In Ref. 9, a predefined latent space transformation operator is used to encourage the topographic organization over time. Beyond the autoencoder-based approaches, Ref. 10 demonstrates the identifiability in nonlinear independent component analysis (ICA) utilizing the temporal structure of data.

Some recent representation learning methods also try to preserve relevant geometric information of data. In Ref. 11, the authors propose a stochastic Riemannian metric to characterize the distortion in the learned latent space. Ref. 12 develops a method based on Isomap to construct an intrinsic and isometric data representation using local Mahalanobis-based distances. Following a similar idea, an autoencoder-based approach is proposed in Ref. 13 for learning an isometric embedding to the latent variables of the manifold.

Another related area is disentangled representation learning. Ref. 14 provides a nice review of the recent progress. Most of these methods purely focus on static properties of the data, but some authors have started to leverage the temporal information in disentanglement.<sup>15,16</sup>

Regarding work in inference of SDEs, in Ref. 17 a data-driven sparse regression method is proposed to discover the governing partial differential equations of a given system with a predefined dictionary of functions, and an innovative spatial and temporal sampling strategy is also used to efficiently handle large data sets. In Ref. 18, this sparse regression framework has been further generalized to stochastic dynamical systems. Ref. 19 introduces an approach for learning non-parametric drift and diffusion functions of SDEs using Gaussian processes, while Ref. 20 reconstructs from a Brownian trajectory the force field and the diffusion field by projecting them onto a finite-dimensional functional space. Ref. 21 generalizes the adjoint sensitivity method to SDEs and achieves competitive performance on inferring latent stochastic dynamics for a high-dimensional dataset.

## SUPPLEMENTARY REFERENCES

- <sup>1</sup>H. J. Berendsen, D. van der Spoel, and R. van Drunen, Computer physics communications **91**, 43 (1995).
- <sup>2</sup>M. J. Abraham, T. Murtola, R. Schulz, S. Páll, J. C. Smith, B. Hess, and E. Lindahl, SoftwareX **1**, 19 (2015).
- <sup>3</sup>G. A. Tribello, M. Bonomi, D. Branduardi, C. Camilloni, and G. Bussi, Computer Physics Communications **185**, 604 (2014).
- <sup>4</sup>G. Bussi, D. Donadio, and M. Parrinello, The Journal of chemical physics **126**, 014101 (2007).
- <sup>5</sup>S. Lameh, L. Ding, and D. Stein, Physical Review Applied **14**, 054042 (2020).
- <sup>6</sup>A. Hasan, J. M. Pereira, S. Farsiu, and V. Tarokh, IEEE Transactions on Signal Processing (2021).
- <sup>7</sup>J.-H. Prinz, H. Wu, M. Sarich, B. Keller, M. Senne, M. Held, J. D. Chodera, C. Schütte, and F. Noé, The Journal of chemical physics **134**, 174105 (2011).
- <sup>8</sup>C. Yildiz, M. Heinonen, and H. Lahdesmaki, Advances in Neural Information Processing Systems **32** (2019).
- <sup>9</sup>T. A. Keller and M. Welling, arXiv preprint arXiv:2109.01394 (2021).
- <sup>10</sup>A. Hyvarinen and H. Morioka, Advances in Neural Information Processing Systems **29**, 3765 (2016).
- <sup>11</sup>G. Arvanitidis, L. K. Hansen, and S. Hauberg, arXiv preprint arXiv:1710.11379 (2017).
- <sup>12</sup>A. Schwartz and R. Talmon, SIAM Journal on Imaging Sciences **12**, 1347 (2019).
- <sup>13</sup>E. Peterfreund, O. Lindenbaum, F. Dietrich, T. Bertalan, M. Gavish, I. G. Kevrekidis, and R. R. Coifman, Proceedings of the National Academy of Sciences **117**, 30918 (2020).
- <sup>14</sup>F. Locatello, S. Bauer, M. Lucic, S. Gelly, B. Schölkopf, and O. Bachem, arXiv preprint arXiv:1811.12359 (2019).
- <sup>15</sup>D. Klindt, L. Schott, Y. Sharma, I. Ustyuzhaninov, W. Brendel, M. Bethge, and D. Paiton, arXiv preprint arXiv:2007.10930 (2020).
- <sup>16</sup>J.-T. Hsieh, B. Liu, D.-A. Huang, L. F. Fei-Fei, and J. C. Niebles, Advances in neural information processing systems **31** (2018).
- <sup>17</sup>S. H. Rudy, S. L. Brunton, J. L. Proctor, and J. N. Kutz, Science advances **3**, e1602614 (2017).

- <sup>18</sup>L. Boninsegna, F. Nüske, and C. Clementi, The Journal of chemical physics **148**, 241723 (2018).
- <sup>19</sup>C. Yildiz, M. Heinonen, J. Intosalmi, H. Mannerstrom, and H. Lahdesmaki, in 2018 IEEE 28th International Workshop on Machine Learning for Signal Processing (MLSP) (IEEE) pp. 1–6.
- <sup>20</sup>A. Frishman and P. Ronceray, Physical Review X **10**, 021009 (2020).
- <sup>21</sup>X. Li, T.-K. L. Wong, R. T. Chen, and D. Duvenaud, in International Conference on Artificial Intelligence and Statistics (PMLR) pp. 3870–3882.
